# Supplementary material for: Privacy Risks in Reinforcement Learning for Household Robots
Source: arXiv:2306.09273 source file (2024-12-06)
Supplement: Supplementary file 1 [file appendix.tex]

\section{DQN Model Structure}
\label{app:network}

\begin{figure}[h]
    \centering
    \includegraphics[width=1.0\textwidth]{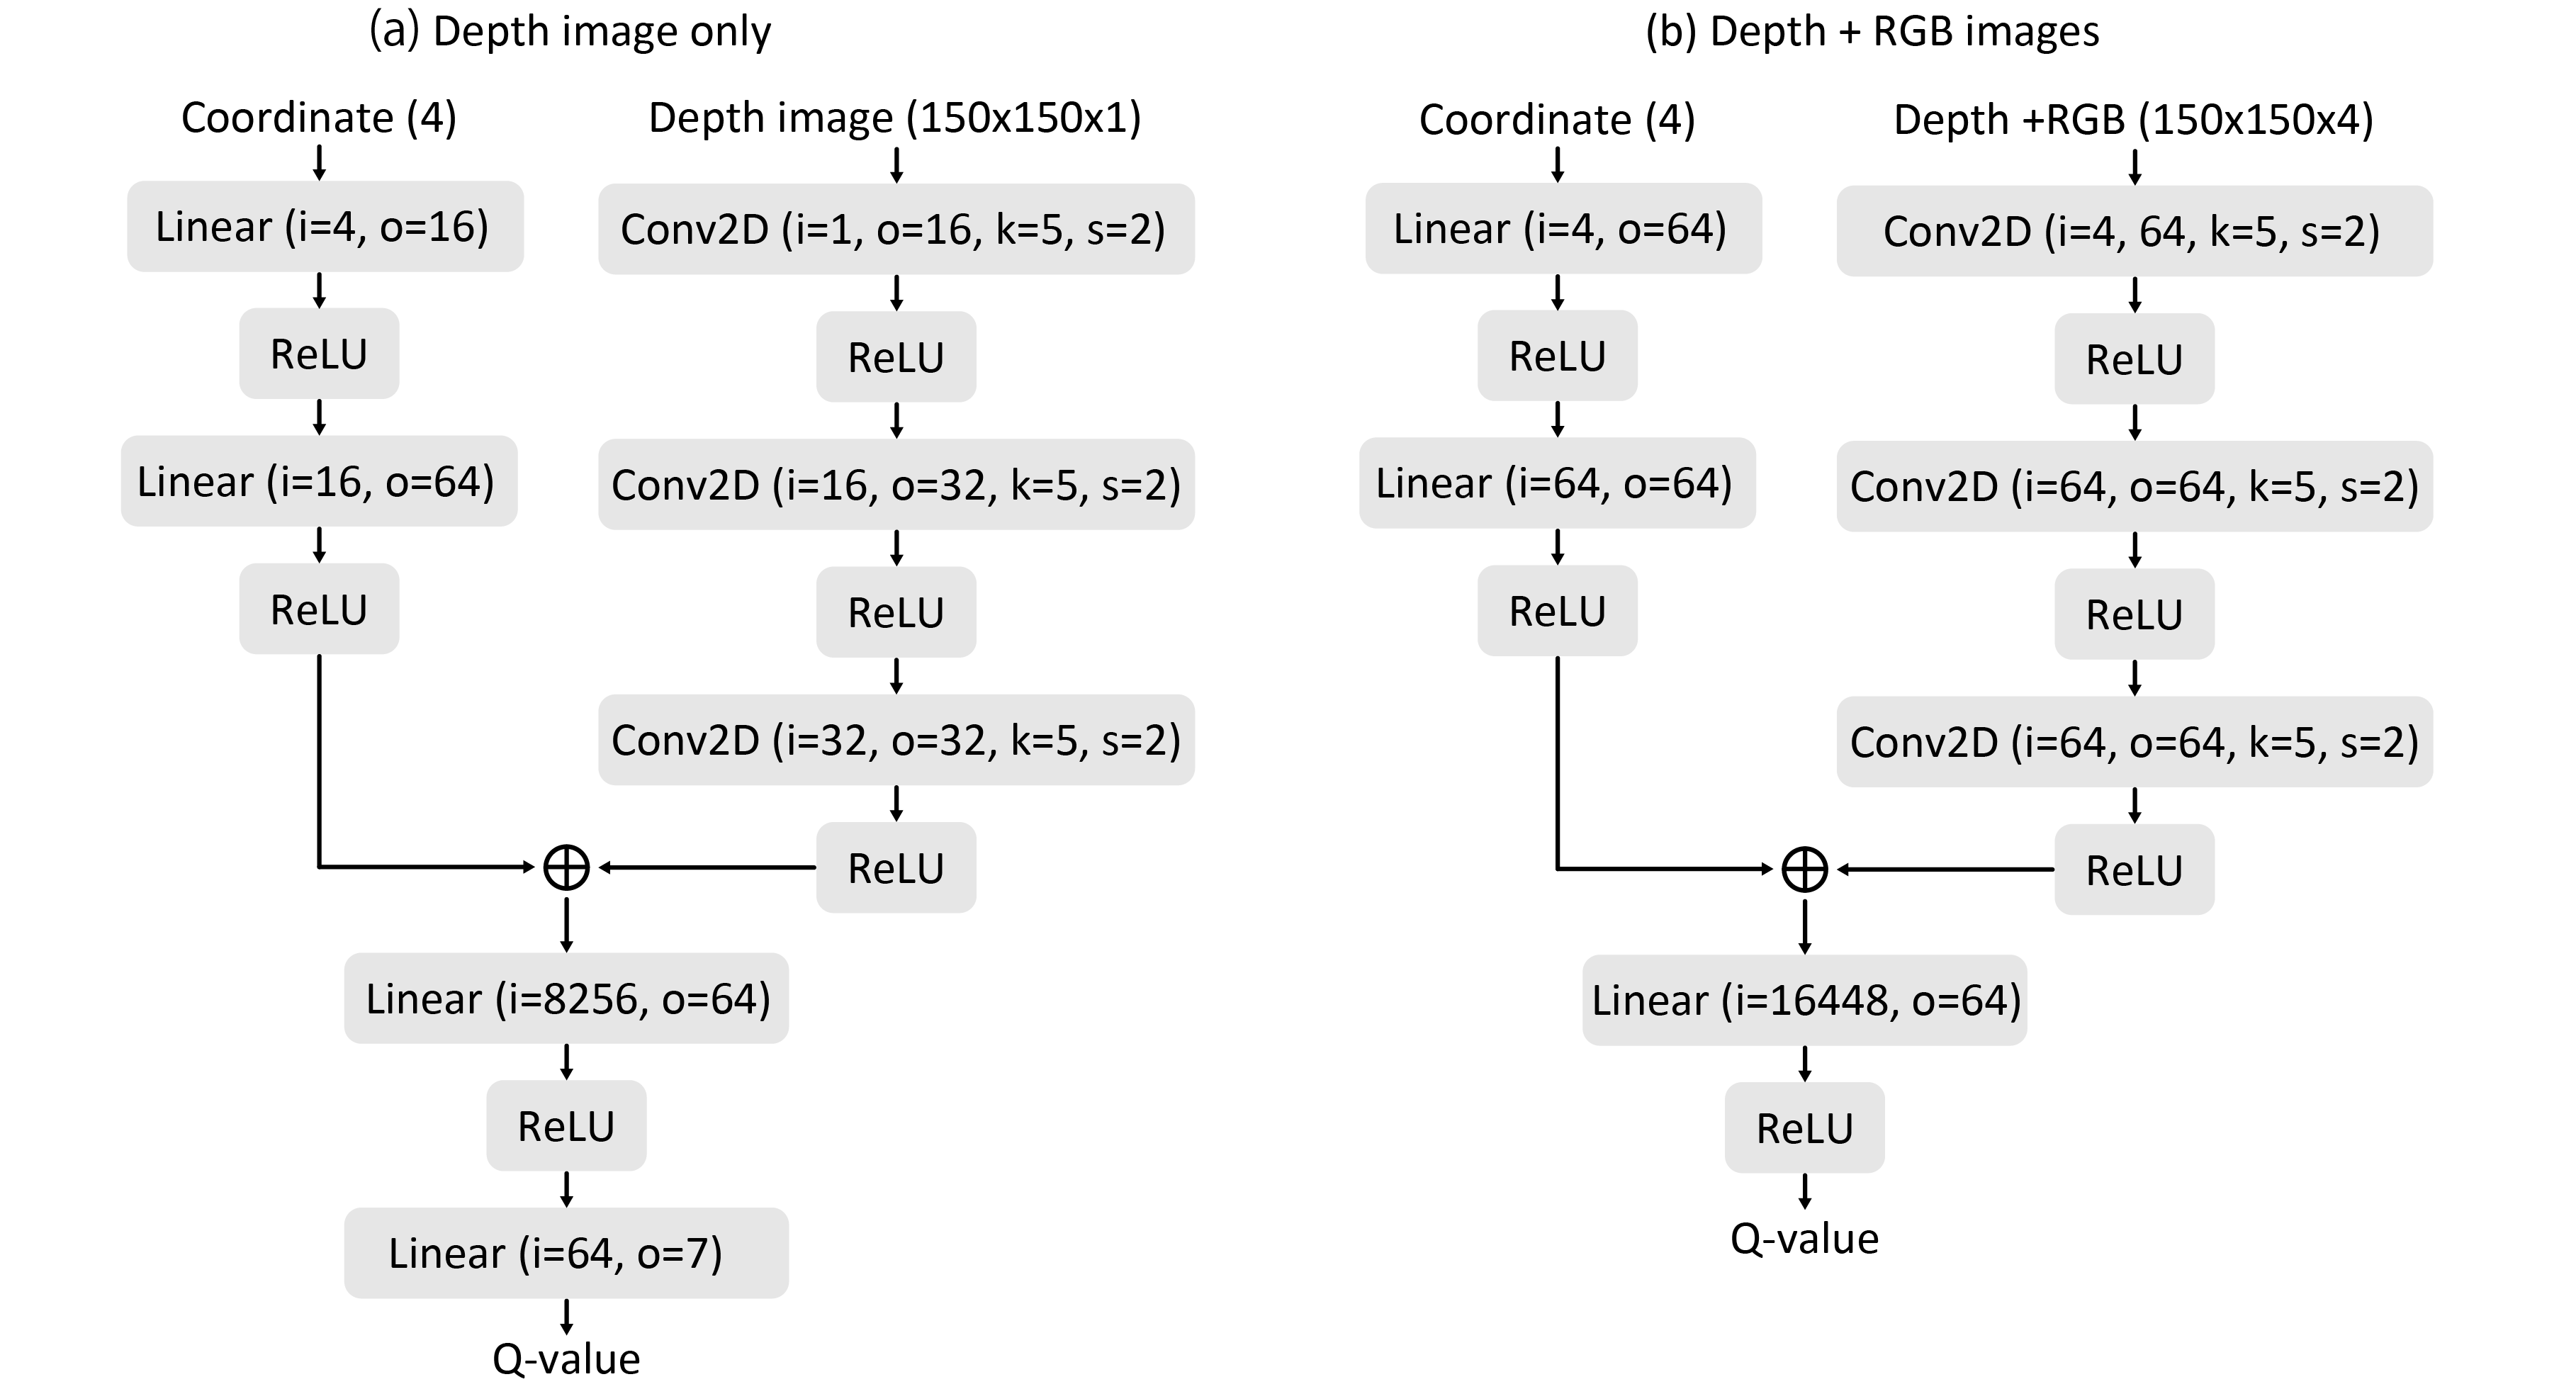}
    \caption{The model structure of the depth-only network and the depth+RGB network.}
    \label{fig:network_structure}
\end{figure}

\section{More Experimental Results}
\label{app:more_results}

\begin{figure}[h]
    \centering
    \includegraphics[width=0.95\textwidth]{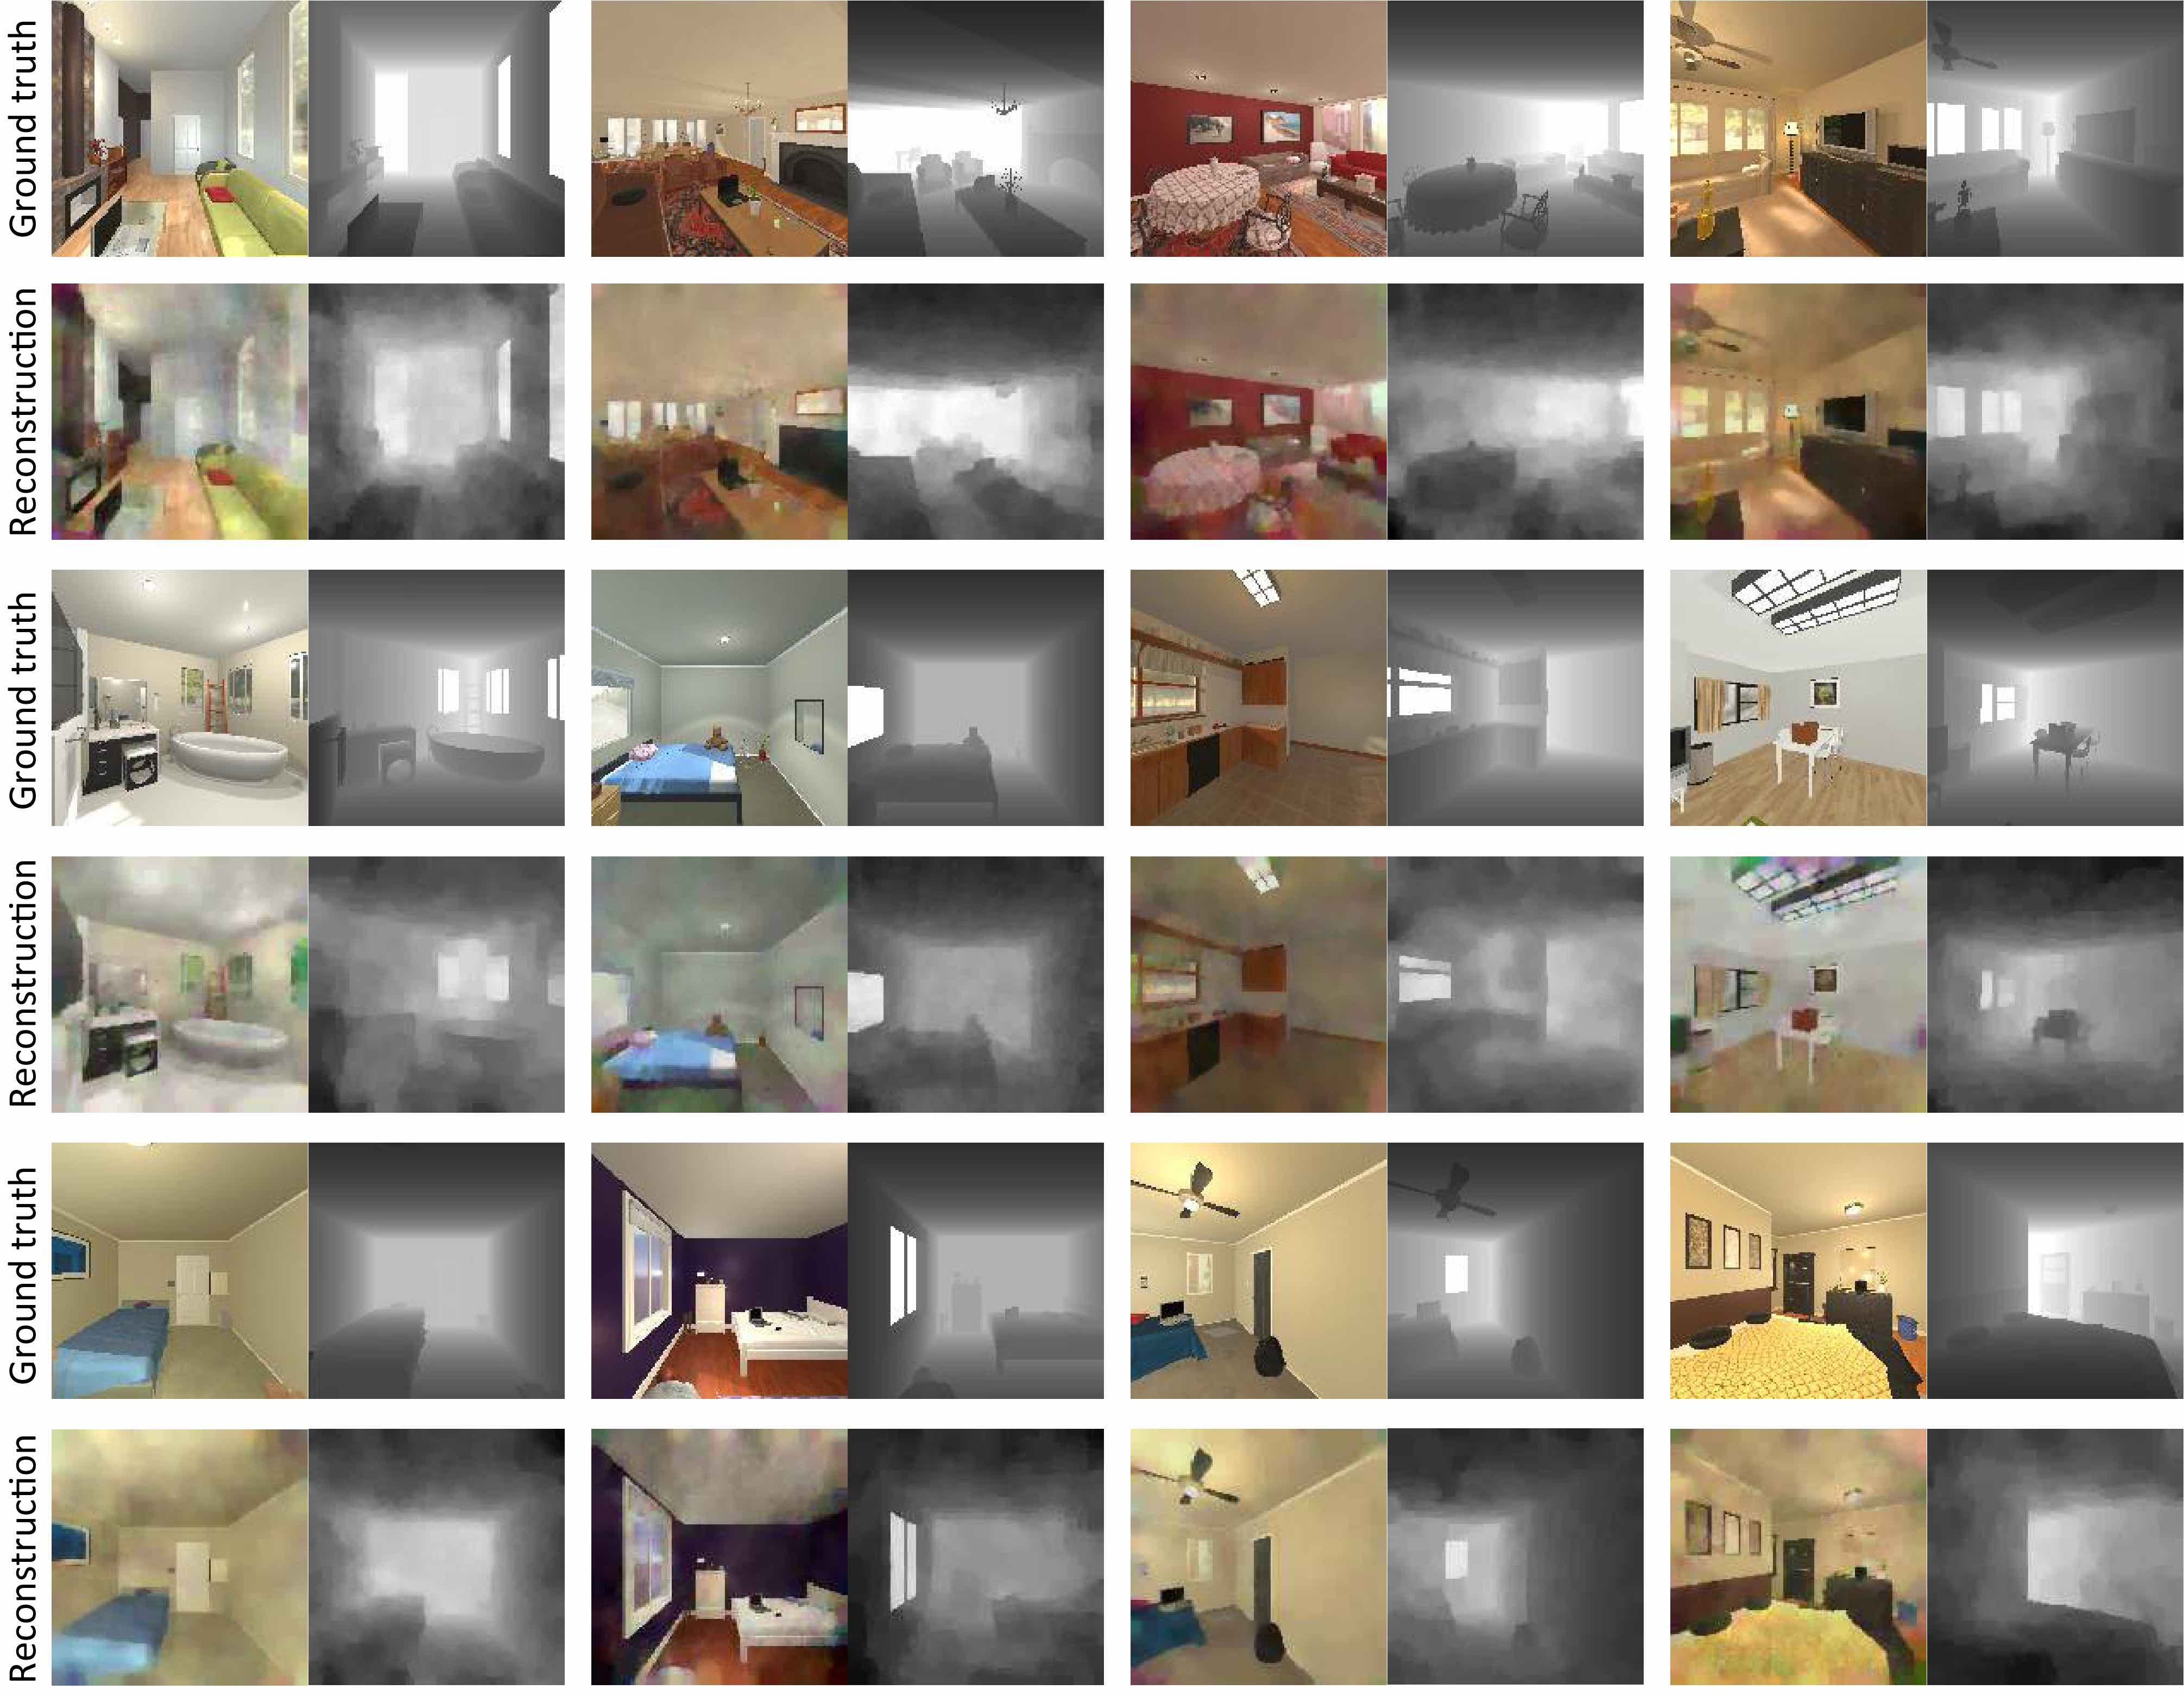}
    \caption{More qualitative results of the depth+RGB image (S1)setting.}
    \label{fig:more_rgb_results}
\end{figure}

We demonstrate more qualitative results of the depth+RGB image setting and the depth-only image setting in Figure~\ref{fig:more_rgb_results} and Figure~\ref{fig:more_depth_results}, respectively.

\begin{figure}[h]
    \centering
    \includegraphics[width=1.0\textwidth]{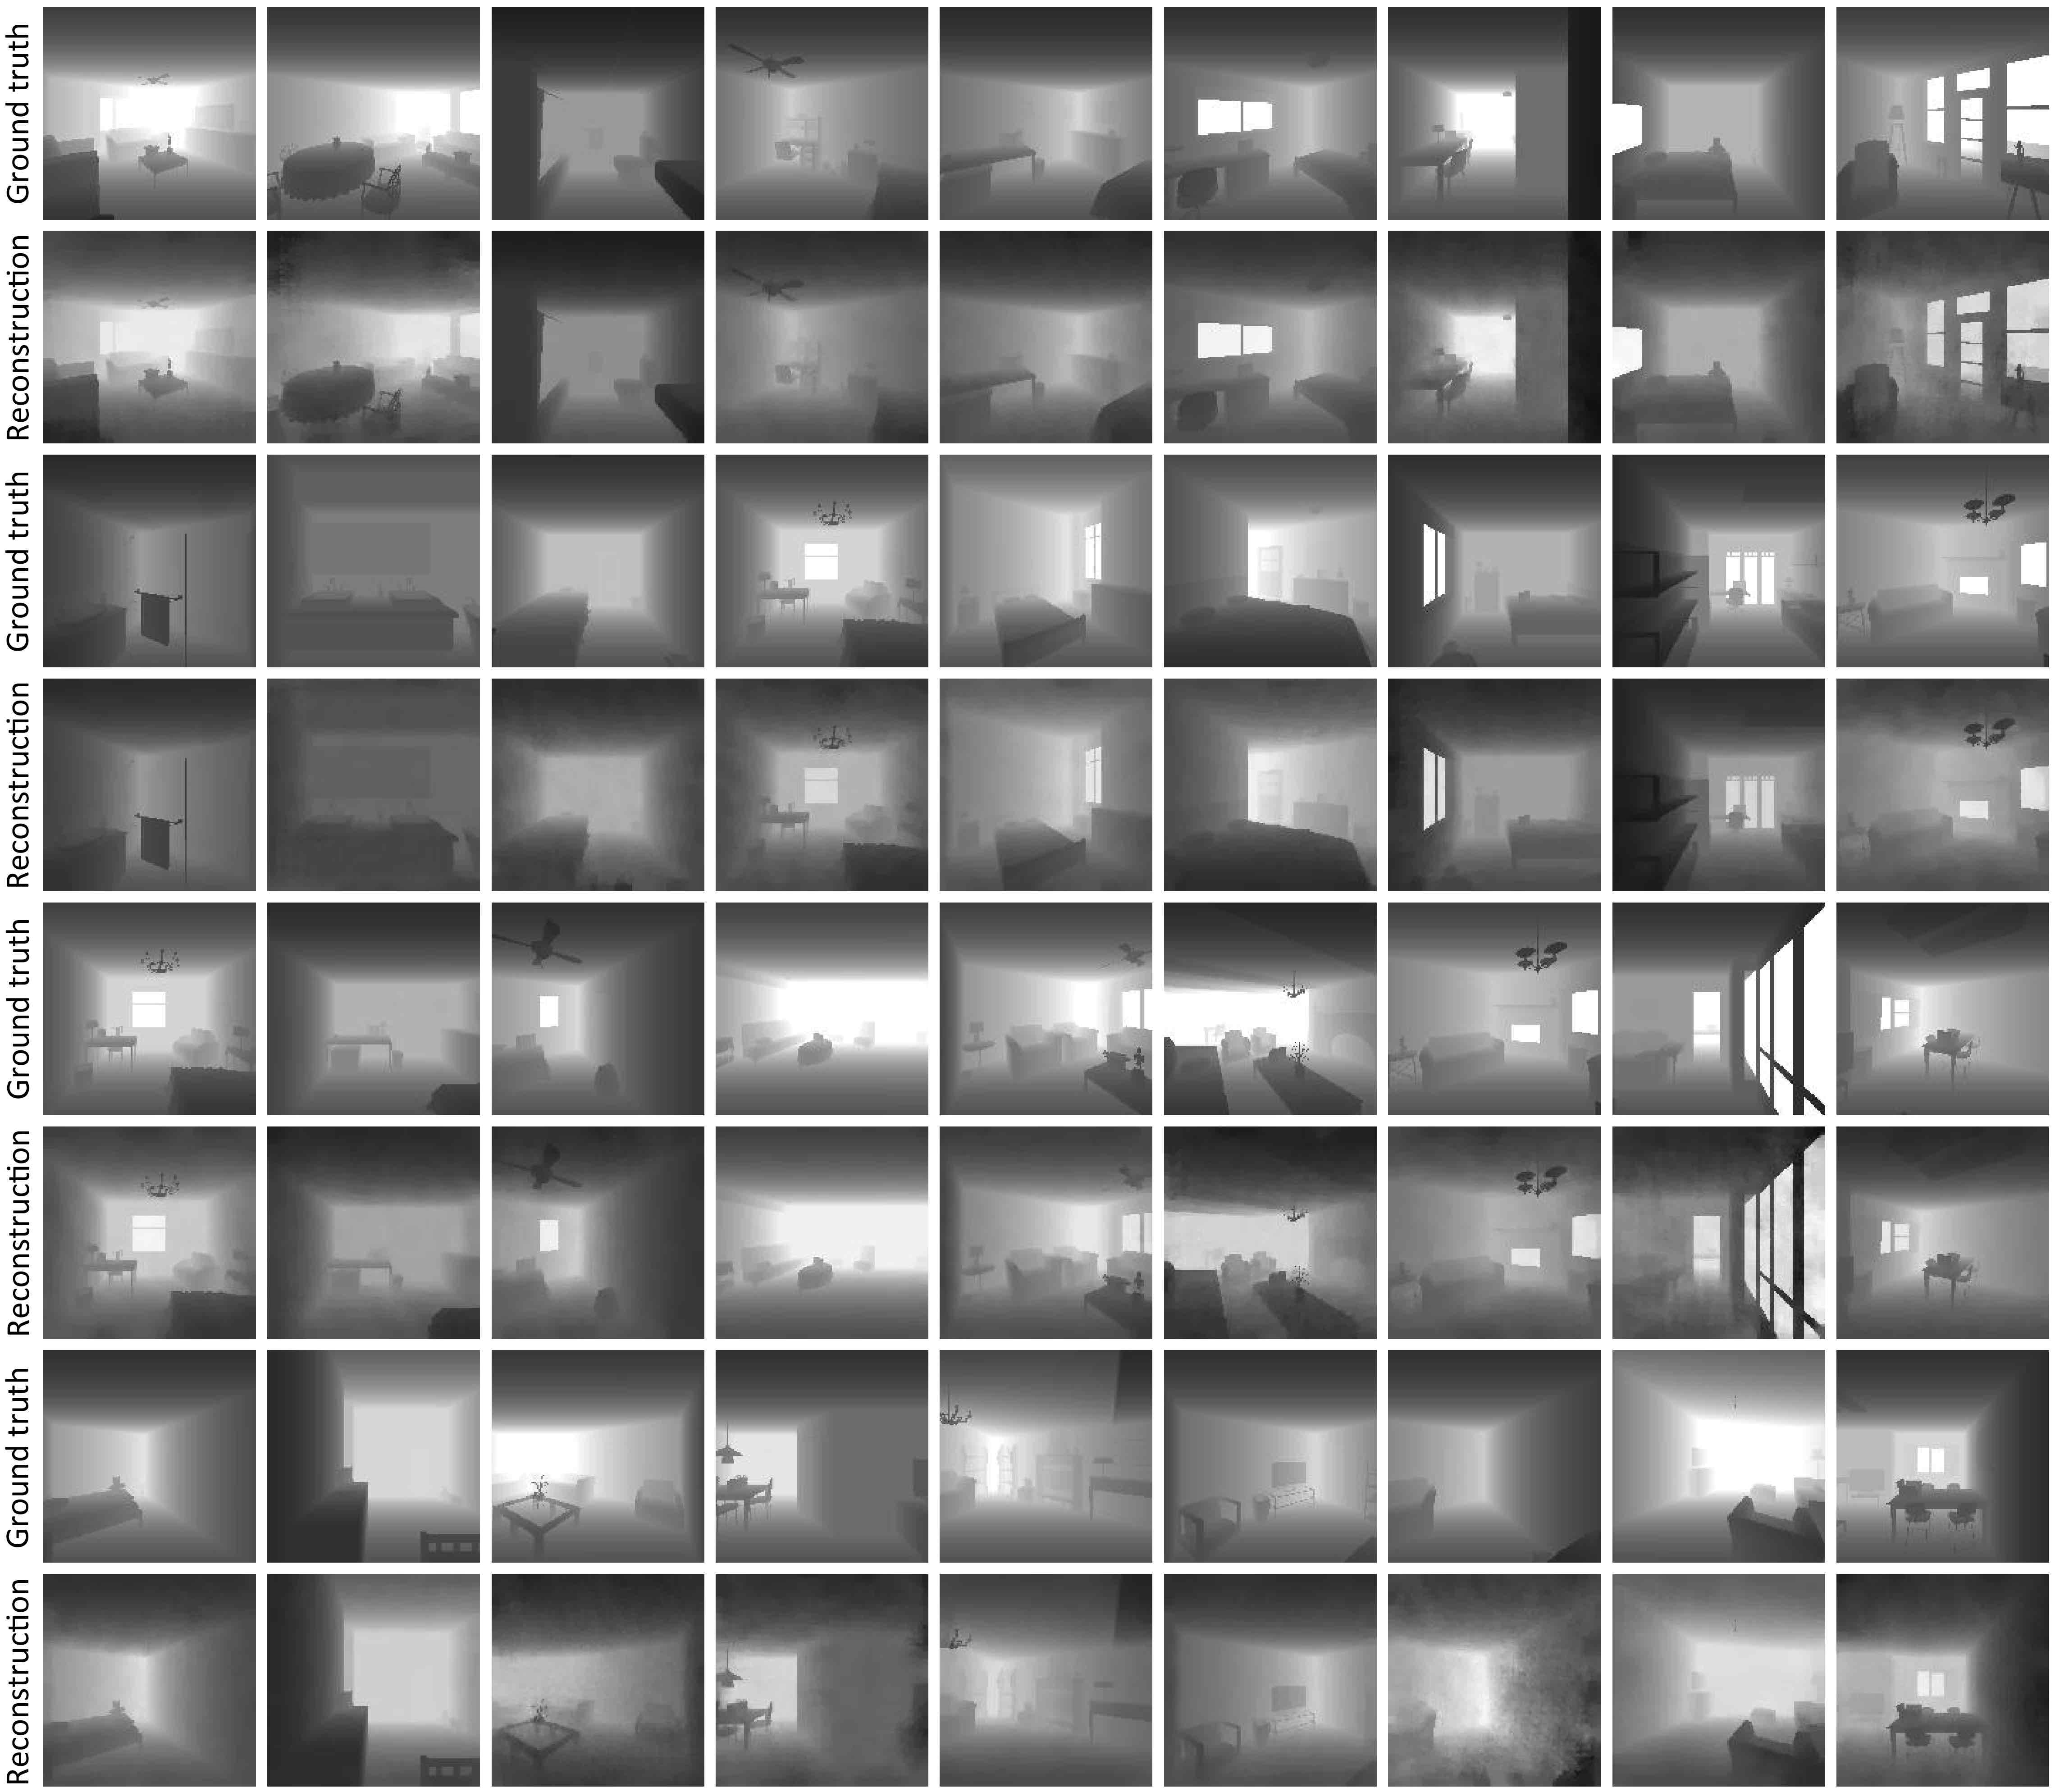}
    \caption{More qualitative results of the depth-only image (S2) setting.}
    \label{fig:more_depth_results}
\end{figure}

We also investigate the possibility of gradient inversion on a \textbf{trained} network.
Figure \ref{fig:trained_depth_results} shows depth image reconstruction from gradients of a trained DQN, which demonstrates some of the most recognizable results. The edges and details are reconstructed with high fidelity and depth estimations are comparable with the ground truth.

The gradient matching loss values are shown in Table \ref{tab:gradient matching loss}.
Specifically, we record the smallest gradient matching loss for each sample during the iteration and calculate the mean and standard derivative.
As shown in the first and second rows, the gradient matching loss values of the vector state reconstruction are much smaller than the image reconstruction stage, consistent with the statement that gradient inversion of the convolution layer is more challenging than the linear layer. 
Note that the vector reconstruction stage results of the S1 are smaller than the results in the S2 because the network used in thing S1 has more parameters than the network used in the S2 setting, providing more information about the training data.
For the image reconstruction stage, the loss values of S1 are larger than the S2, indicating the reconstruction of both RGB and depth images is more challenging than reconstructing only the depth image, due to the larger dimension of data.
\begin{table}[h]
    \centering
    \caption{Gradient Matching Loss for vector state reconstruction and image state reconstruction.}
    \scalebox{0.9}{
    \begin{tabular}{c|cc}
        \toprule
        method  & vector state reconstruction &  image state reconstruction  \\
        \midrule
        QGI (S2) & $1.206\times10^{-5}\pm1.139\times10^{-4}$ & $7.364\times10^{-4}\pm1.462\times10^{-3}$   \\
        
        QGI (S1)  & $7.778\times10^{-7}\pm1.058\times10^{-5}$ & $2.518\times10^{-3}\pm 2.129$  \\
        
        joint (S1) & \multicolumn{2}{c}{$2.094\times10^{-3}\pm1.385\times10^{-3}$} \\
        \bottomrule
    \end{tabular}}
    \label{tab:gradient matching loss}
\end{table}
\begin{figure}[h]
    \centering
    \includegraphics[width=1.0\textwidth]{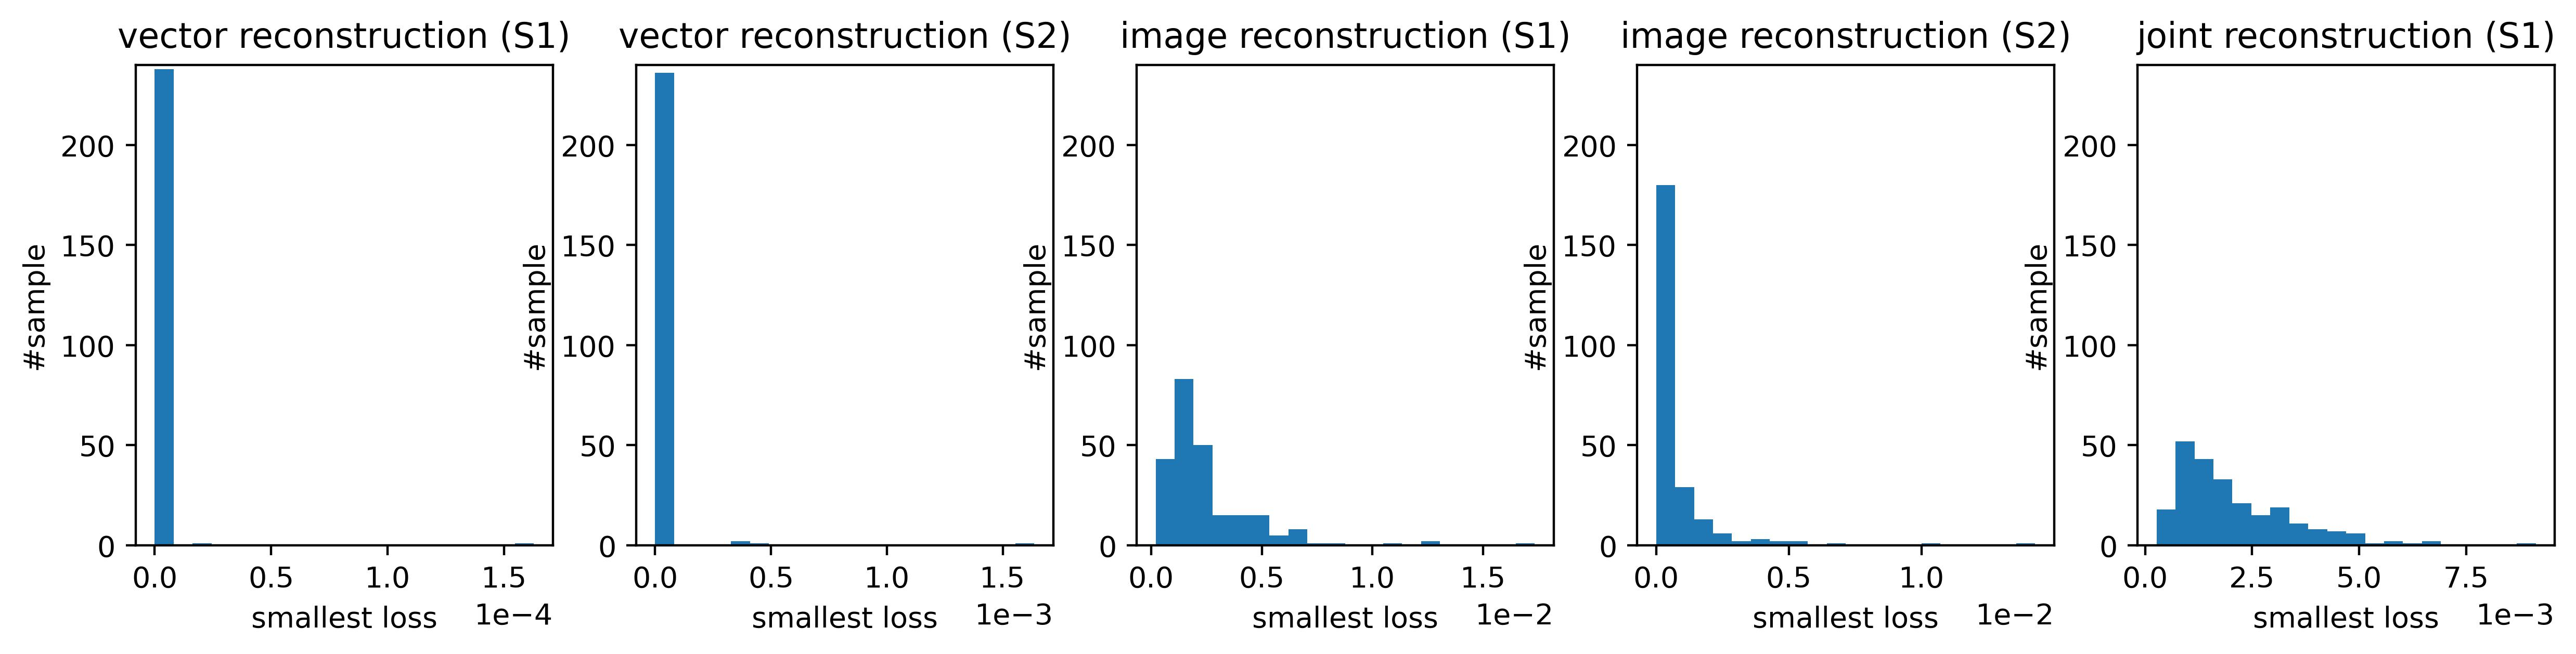}
    \caption{Histogram of smallest gradient matching loss values for state reconstruction in S1 and S2 settings.}
    \label{fig:smallest loss hist}
\end{figure}
As shown in Figure \ref{fig:smallest loss hist}, 235(S1) and 228(S2) out of the 240 samples have the smallest gradient matching loss reaching 0 in the vector state reconstruction stage, while in the image state reconstruction stage, no gradient matching loss can converge to 0.
Although joint optimization achieves a smaller mean result than the proposed QGI, as shown in Table \ref{tab:gradient matching loss}, the histogram shows that QGI tends to generate reconstructions with small gradient matching losses, while joint optimization of vector and joint results in more large results.

\begin{figure}[h]
    \centering
    \includegraphics[width=1.0\textwidth]{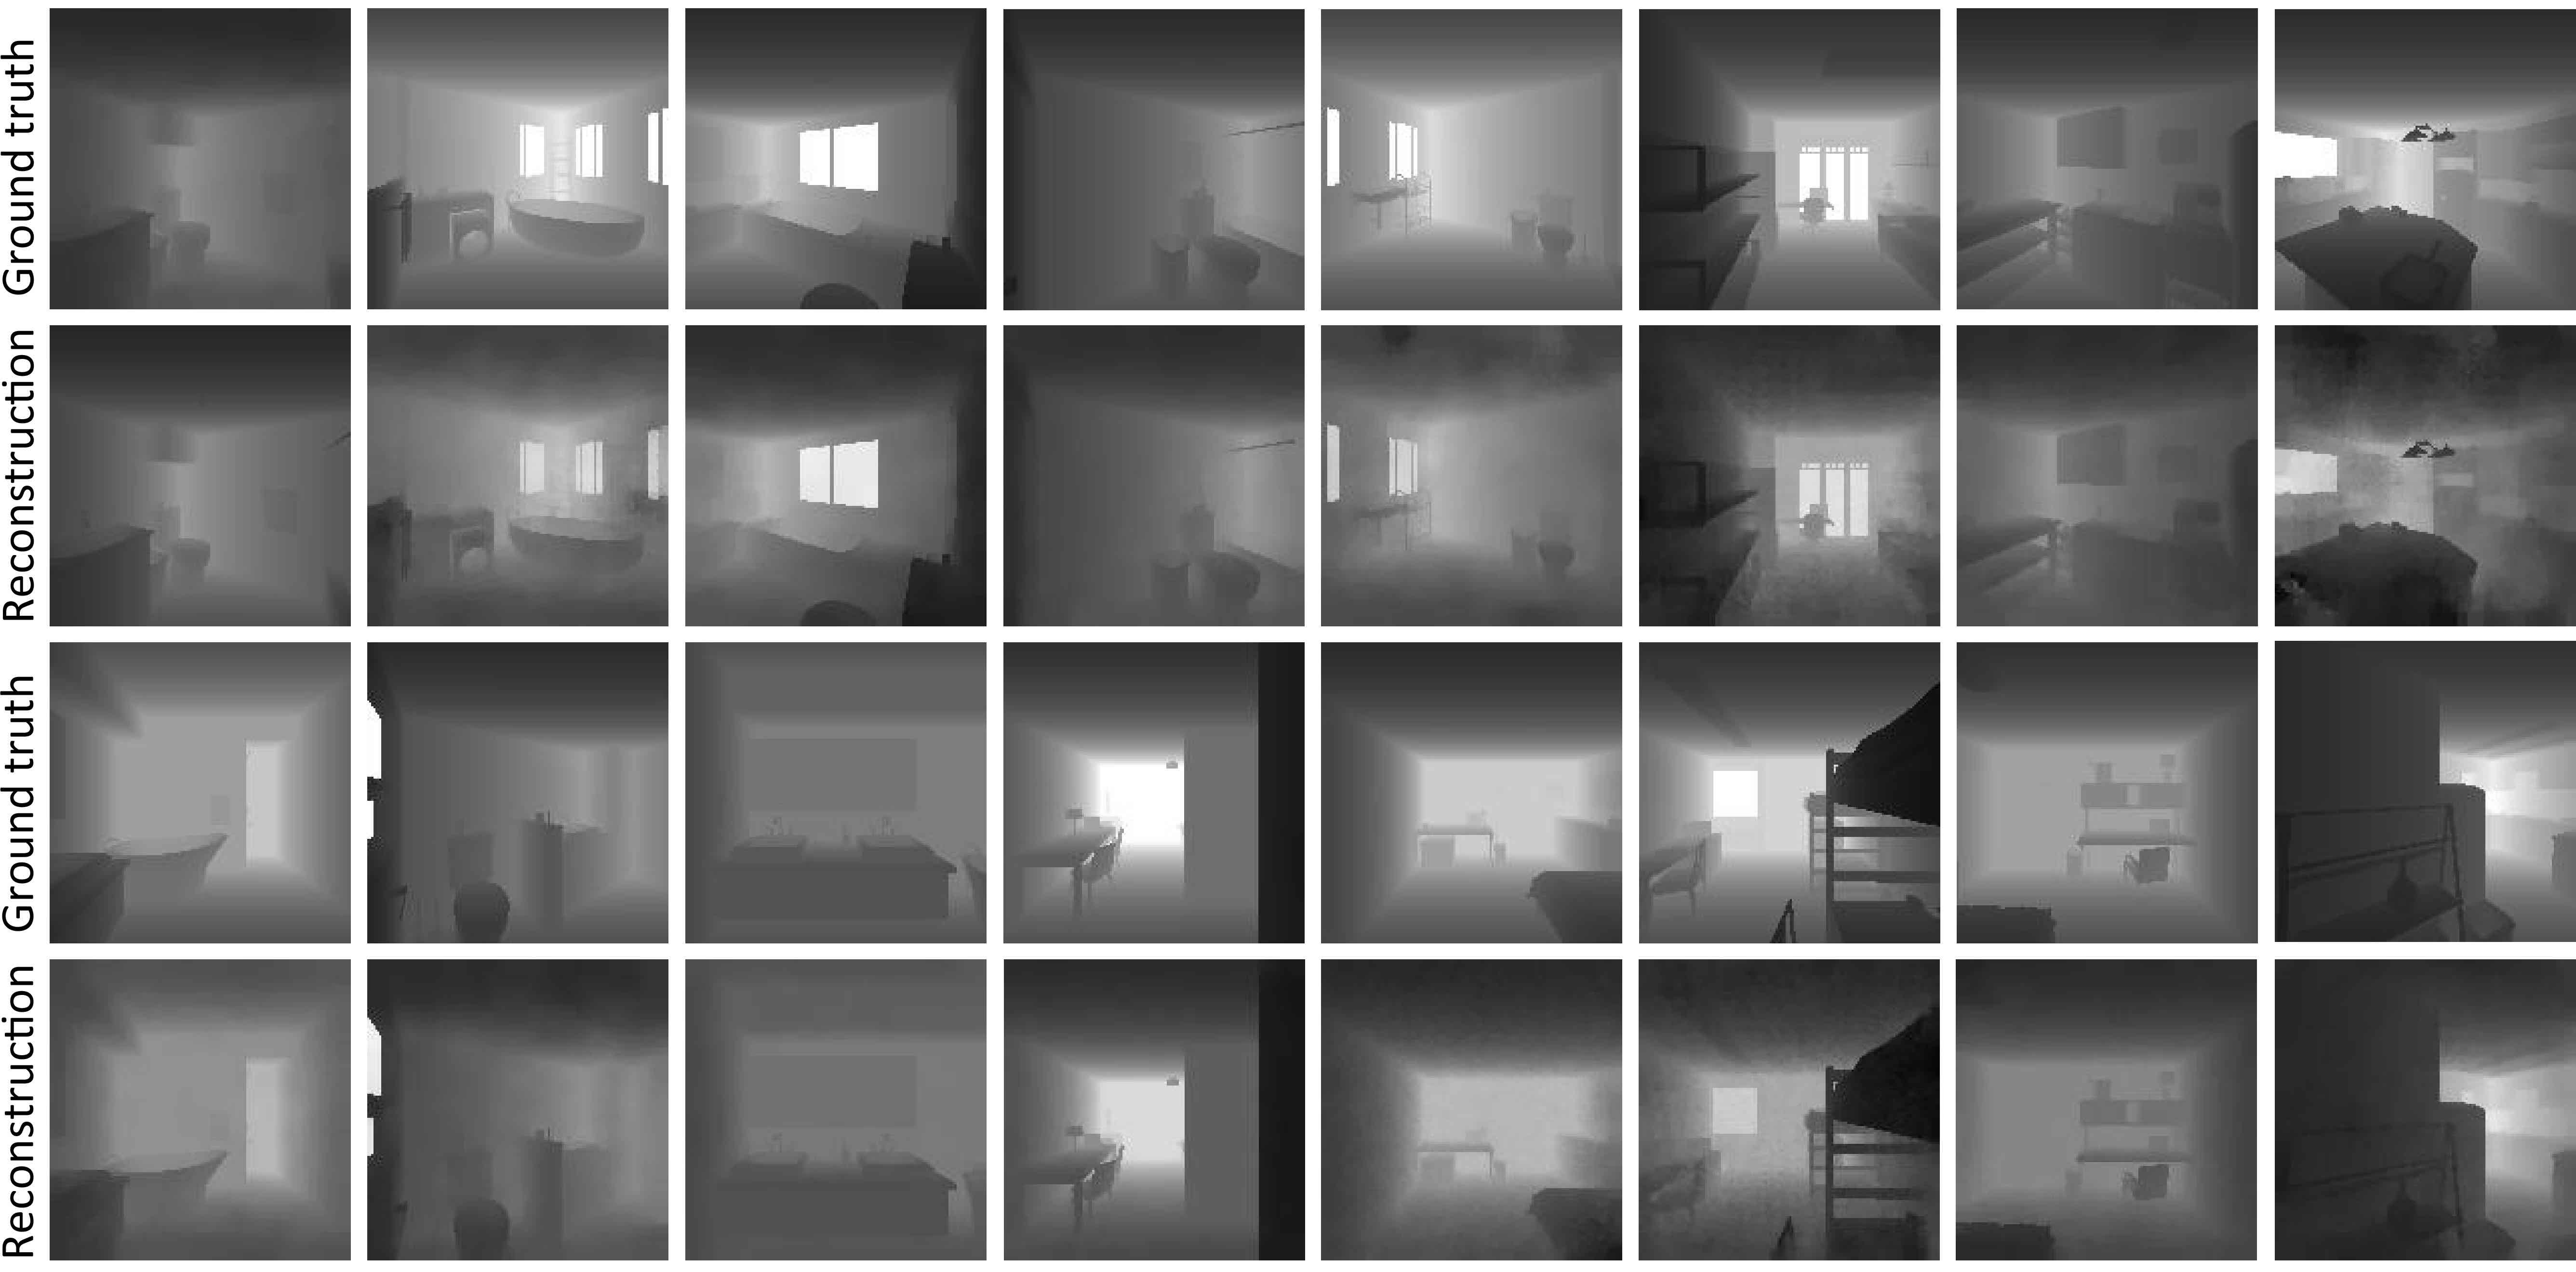}
    \caption{Qualitative results of depth images (S2) on trained DQN.}
    \label{fig:trained_depth_results}
\end{figure}

\section{Experiment Settings}
\label{app:experiment_settings}
The optimization is conducted by AdamW optimizer with betas$=(0.9,0.999)$.
The learning rate is initialized to 0.1 and decays during the iteration.
For the vector state reconstruction, the learning rate decays by 10 times at iteration $8\times10^3$ and $1.6\times10^4$. 
For the image state reconstruction, the learning rate decays by 10 times at iteration $4\times10^3$, $1\times10^4$, and $1.6\times10^4$. 
We find the update of the state is unstable and thus, we only preserve the sign of the state gradient, for example, $\text{sign}(\frac{\partial L}{\partial s_c})$ to use as final gradient passing to the optimizer.
We also clip the reconstructed image state $s_i^{rec}$ and $s_d^{rec}$ in every iteration to force the search space lying inside $[0,1]^{150\times 150}$.
The final vector state reconstruction is selected by locating the smallest gradient matching loss.
The final image state is selected by locating the smallest gradient matching loss and the smallest TV loss, resulting in 2 image reconstructions for each image state.
To obtain the quantitative result, the same evaluation is conducted for the 2 images, and the better one is used for the mean, standard derivative, and maximum value calculation.
Note that the 2 reconstructed images are considerably similar.
Moreover, the adversary can retrieve both images to steal private information and our goal is to demonstrate the potential risk.

All of our experiments are conducted on a machine with 2$\times$ AMD EPYC 7542 32-Core CPU, an NVIDIA RTX A6000 GPU (48GB memory), and 256GB memory.

\section{More Explanation on Method}
\label{explanation:sign Q}
Gradient inversion aims to reconstruct the training data by optimizing the reconstructed data to mimic the true gradient.
Given the Q-network, the gradient is 
\begin{align}
    g &= \frac{\partial J(\hat{Q},Q)}{\partial \hat{Q}} \frac{\partial \hat{Q}}{\partial w} = 2(\hat{Q}-Q)\frac{\partial \hat{Q}}{\partial w}.
    \label{eq:gradient}
\end{align}
The gradient contains 2 components, namely $2(\hat{Q}-Q)$ and $\frac{\partial \hat{Q}}{\partial w}$.
A sufficiently accurate estimation of the first term can accelerate the optimization of the gradient matching loss, specifically, mimicking the second term by reconstructing the training data.
We find in experiments that an accurate $2(\hat{Q}-Q)$ reconstruction is more beneficial than an accurate supervision signal $Q$ reconstruction.
Moreover, observing that the magnitude of $\hat{Q}-Q$ has no influence on the gradient matching loss $L$, we propose to first reconstruct the sign $\Vec{n}=\hat{Q}-Q$, and use the reconstructed sign in the reconstruction of the vector and the image state. 
The usage of $\Vec{n}$ during the state reconstruction is conducted by defining a constant $\tilde{Q}$ as the temporary reconstruction of the target Q-value, which is sufficiently large and thus the reconstructed error $\hat{Q}^{rec}-\tilde{Q}$ has the sign $\Vec{n}$.

\begin{table*}
    \centering
    \begin{tabular}{c|c|ccccccc}
    \toprule
    method & Metric & bathroom & bedroom & kitchen & living room & average & best \\
    \midrule
    \multirow{2}{*}{DQN} & PSNR & ${31.61\pm7.30}$ & ${27.53\pm7.41}$ & ${29.82}\pm8.39$ & {$25.13\pm7.02$} & ${28.52\pm7.89}$ & {48.24} \\
    & SSIM & ${0.949\pm0.049}$ & ${0.916\pm0.049}$ & ${0.923\pm0.078}$ & $0.882\pm0.137$ & ${0.918\pm0.095}$ & {0.998} \\
    \midrule
    \multirow{2}{*}{REINFORCE} &PSNR & $37.49\pm7.28$ & $35.76\pm6.87$ & $35.75\pm5.74$ & $33.72\pm6.83$ & $35.68\pm6.80$ & 57.55 \\
    & SSIM & $0.936\pm0.088$ & $0.912\pm0.109$ & $0.933\pm0.090$ & $0.901\pm0.132$ & $0.923\pm0.106$ & 0.999\\
    \bottomrule
    \end{tabular}
    \caption{after submission}
\end{table*}
